# Supplementary material for: Variational Clustering: Leveraging Variational Autoencoders for Image Clustering
Source: arXiv:2005.04613 source file (2020-05-10)
Supplement: Supplementary file 1 [file results.tex]

\subsection{Toy Data}
\label{ssec:app_toy}

We show the latent space learnt by our method \& GMVAE on the synthetic dataset proposed in their paper. As seen below, our clusters are tightly packed individually \& more spread overall compared to GMVAE. Good latent space separation is key for clustering as we want a representation where data is better partitioned.
\input{latex_figures/toy_data.tex}

\subsection{Generated Samples from Fashion-MNIST}
Fig. \ref{fig:gen_fashion} shows the generative ability of our method in the case of Fashion-MNIST. As it can be seen, it produces realistic images of the clusters from the dataset. Here, we show generated samples from Fashion-MNIST. Despite a little bit of overlap, each cluster almost uniquely represents a different category in the dataset, even though they are visually similar, like 'sneaker' \& 'sandal' (row 1 \& 7) or 'coat' \& 'pullover' (row 4 \& 5). This shows the discriminatory power of our learnt latent space.
\begin{figure}[h!]
    \centering
    \includegraphics[width=0.5\textwidth]{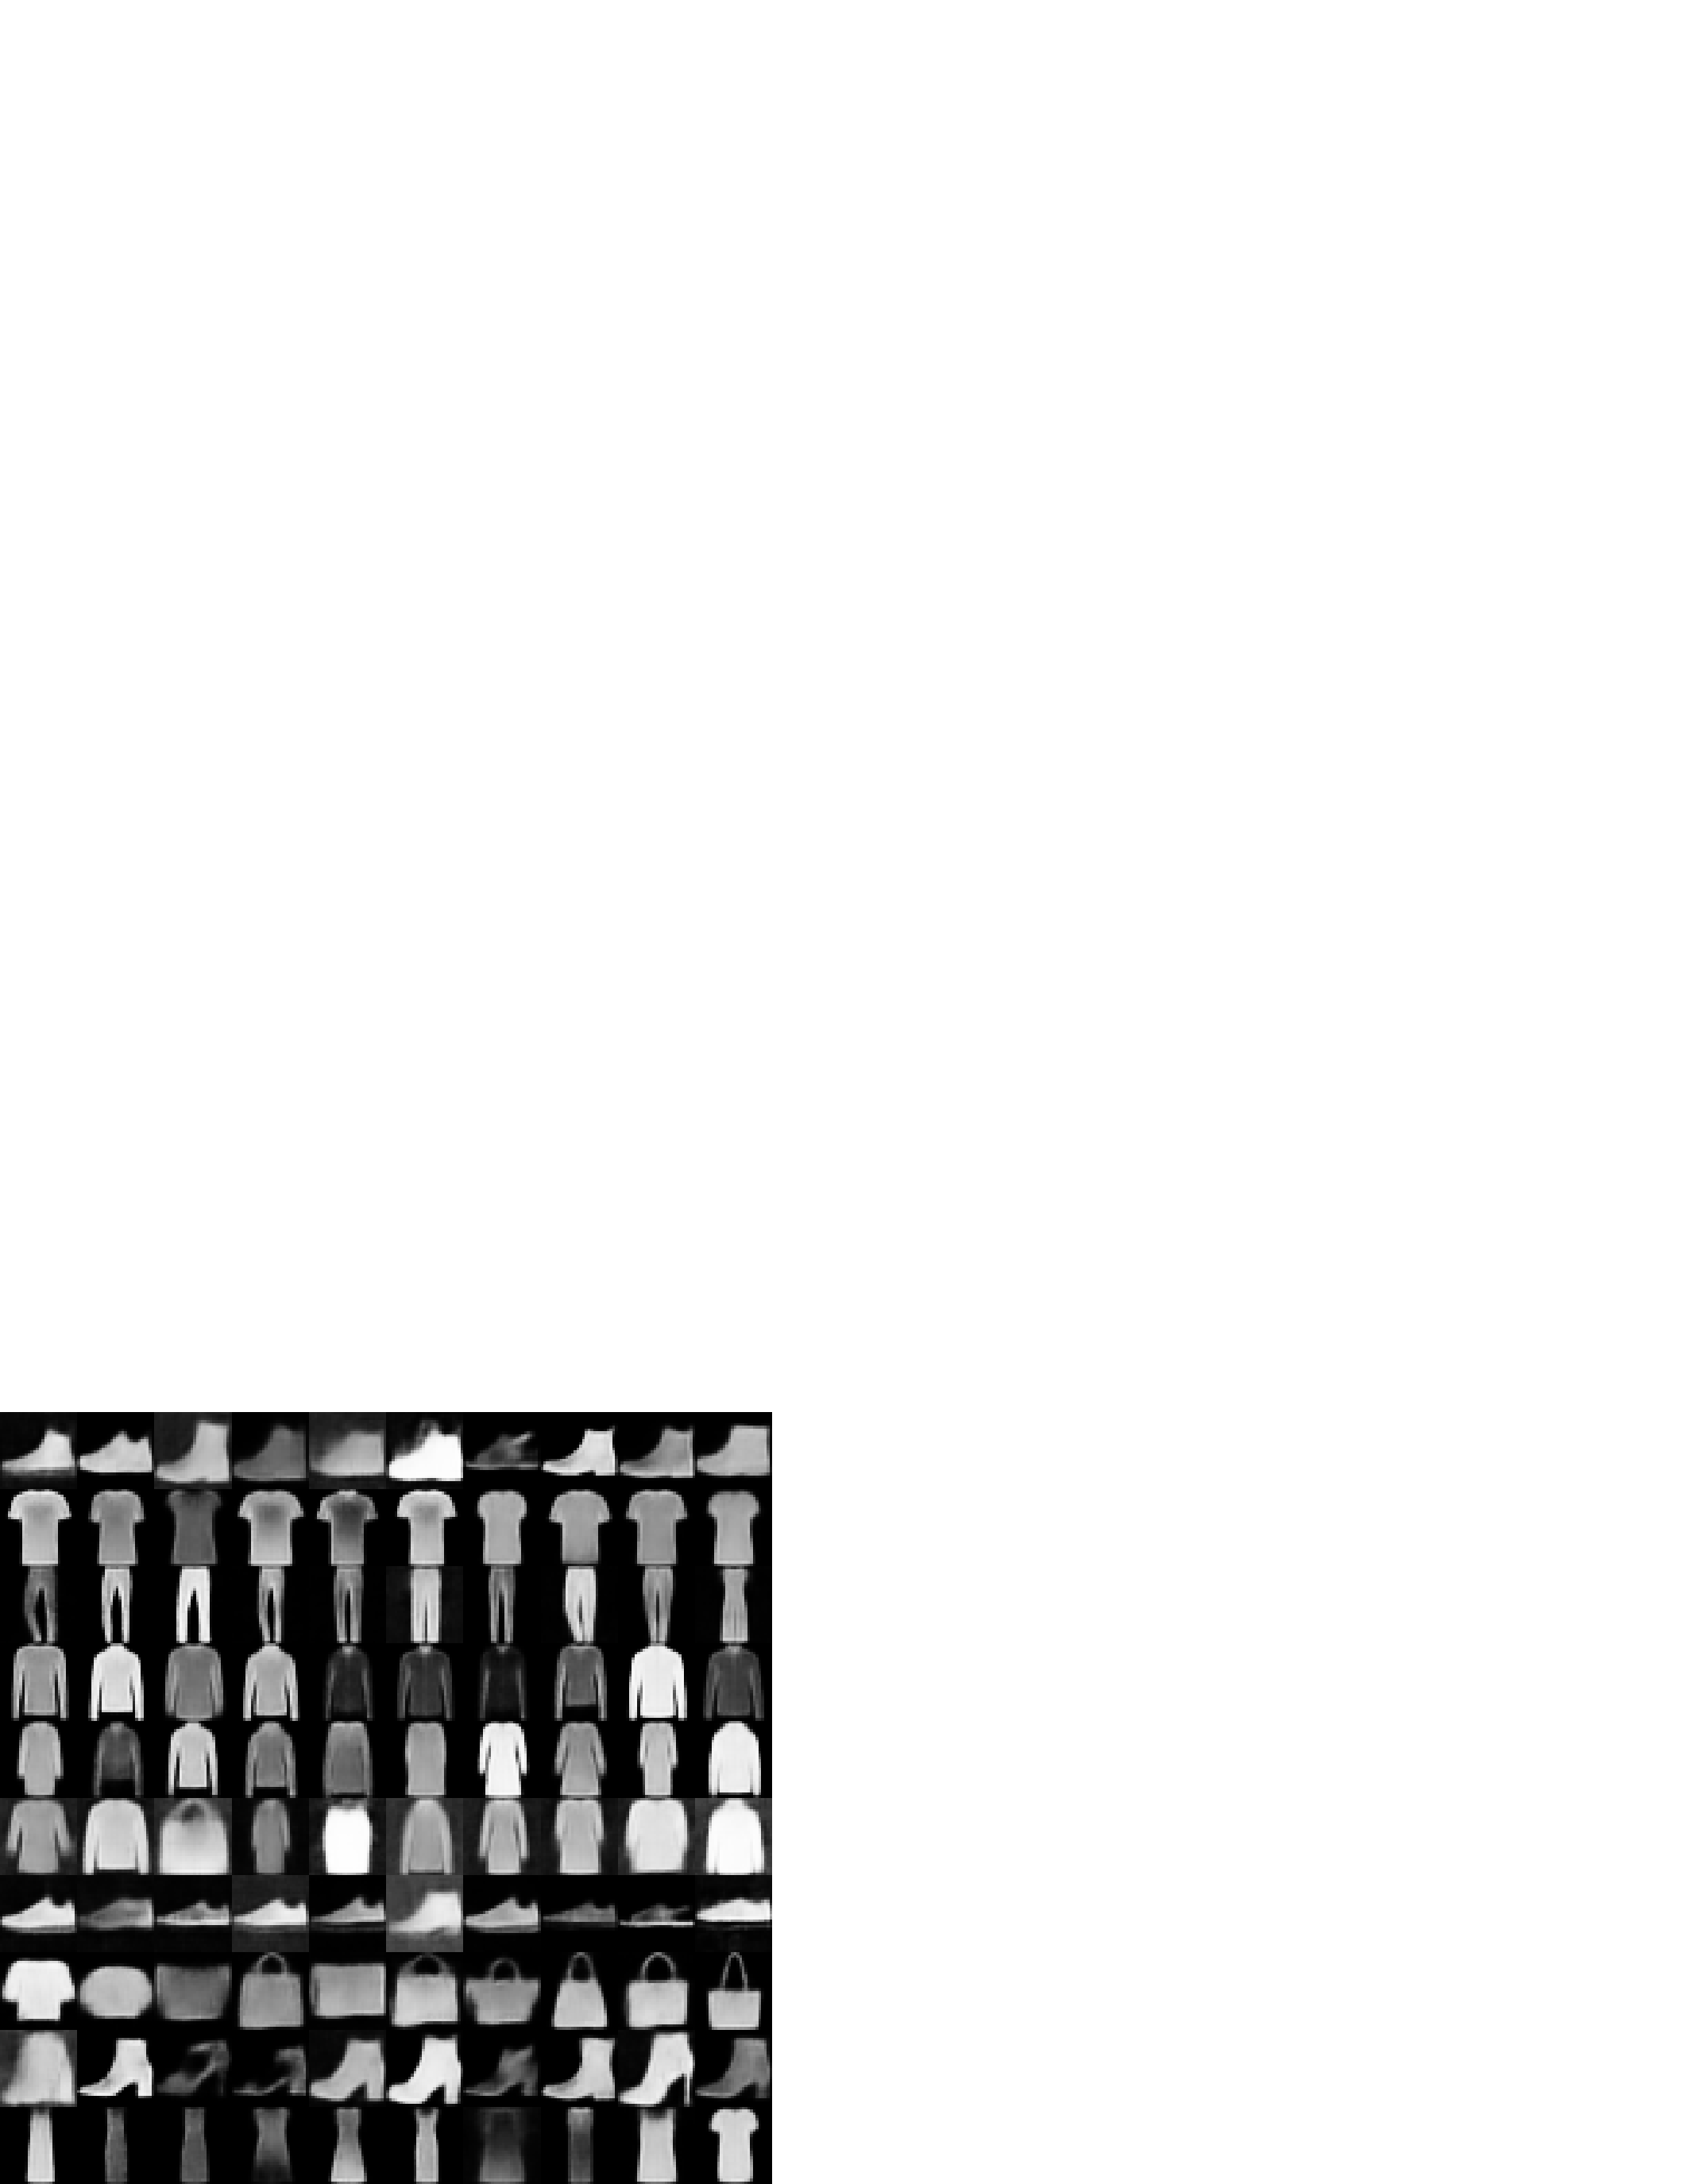}
    \caption{Images generated from each of the clusters in Fashion-MNIST. Each row represents a cluster and each column is an independent Bernoulli distribution generated by $p_\theta(\mathbf{x}|\mathbf{z})$ given a latent $\mathbf{z}$ sampled from the Gaussian Distribution $p_\beta(\mathbf{z}|k)$ corresponding to the $k^{th}$ cluster.}
    \label{fig:gen_fashion}
\end{figure}

\subsection{Best images from STL-10}
In order to see how well our method clusters high dimensional data, we take a look at the top 10 images corresponding to each cluster for STL-10. From Fig. \ref{fig:stl-best} it can be seen that our method is able to distinguish well between similar classes like 'cat' \& 'dog' (row 4 \& 6) and between 'aeroplane' \& 'bird' (row 1 \& 2) where the background is the same (sky) and the structure is similar (head, wings, tail).
\begin{figure}[h!]
    \centering
    \includegraphics[width=0.5\textwidth]{images/stl_best10.png}
    \caption{The top 10 images having highest probability for belonging to each cluster in STL-10.}
    \label{fig:stl-best}
\end{figure}
