# Supplementary material for: Variational Clustering: Leveraging Variational Autoencoders for Image Clustering
Source: arXiv:2005.04613 source file (2020-05-10)
Supplement: Supplementary file 2 [file appendix.tex]

\section{Network Architecture}
\label{sec:app_arch}
\setcounter{figure}{0}
\setcounter{table}{0}
The network architectures for the prior and posterior networks are given in Tables \ref{tab:prior_dist} and \ref{tab:post_dist} respectively. the  $\mathbf{z}$ prior consists of fully connected networks as there aren't any images involved in the process. We share the weights in the convolutional part of the posterior networks for CIFAR10, STL-10, CIFAR100 as they would entail complex representations which can be better captured by sharing the weights. 
\input{latex_tables/nets.tex}

\section{Augmentation Loss}
\label{sec:app_aug}
\setcounter{equation}{0}
The augmentation loss can be written as:
\begin{equation}
\label{eq:aug_loss}
\begin{split}
    \mathcal{L}_{aug} = \sum_{k=1}^K||q_{\phi}(k|\mathbf{x}) - q_{\phi}(k|\mathbf{\hat{x}})||_2^2 \\
    + \mathbb{E}_{q_{\phi}(k|\mathbf{x})}[\mathcal{W}_2(q_{\psi}(\mathbf{z}|\mathbf{x},k), q_{\psi}(\mathbf{\hat{z}}|\mathbf{\hat{x}},k))]
\end{split}
\end{equation}

where $\mathcal{W}_2$ is the 2-Wasserstein distance between the predicted posteriors. The expectation in the latter is due to the fact that we do not know the ground truth cluster to reduce the distance between the prior and posterior of that cluster. Instead, taking the expectation allows us to give a higher weight to the cluster it's predicted to belong to and a lower weight for clusters that are not associated with the given image. 
The 2-Wasserstein distance between the predicted posteriors has a closed form solution\cite{dowson1982frechet} since they are Gaussian distributions, which is given by

\begin{equation}
\label{eq:w_loss}
\begin{split}
    \mathcal{W}_2(q_{\psi}(\mathbf{z}|x,k), q_{\psi}(\mathbf{\hat{z}}|\mathbf{\hat{x}},k)) = ||\mathbf{\mu}_\psi(\mathbf{x},\mathbf{e}_k) - \mathbf{\mu}_\psi(\mathbf{\hat{x}},\mathbf{e}_k)||_2^2\\
     + \hspace{0.2em} trace(C_1 + C_2 - 2(C_2^{\frac{1}{2}}C_1C_2^{\frac{1}{2}})^{\frac{1}{2}})
    % , diag(\mathbf{\sigma}_\psi^2(\mathbf{x},\mathbf{e}_k))
\end{split}
\end{equation}

with $C_1 = diag(\mathbf{\sigma}_\psi^2(\mathbf{x},\mathbf{e}_k))$ and $C_2 = diag(\mathbf{\sigma}_\psi^2(\mathbf{\hat{x}},\mathbf{e}_k))$ in our case. Given this form of $C_1$ and $C_2$, we can simplify $(C_2^{\frac{1}{2}}C_1C_2^{\frac{1}{2}})^{\frac{1}{2}}$ as 
\begin{equation}
\label{eq:C_mult}
\begin{split}
(C_2^{\frac{1}{2}}C_1C_2^{\frac{1}{2}})^{\frac{1}{2}} &= diag(\mathbf{\sigma}_\psi(\mathbf{\hat{x}},\mathbf{e}_k)\mathbf{\sigma}_\psi^2(\mathbf{x},\mathbf{e}_k)\mathbf{\sigma}_\psi(\mathbf{\hat{x}},\mathbf{e}_k))^{\frac{1}{2}}\\
&= diag(\mathbf{\sigma}_\psi(\mathbf{x},\mathbf{e}_k)\mathbf{\sigma}_\psi(\mathbf{\hat{x}},\mathbf{e}_k))
\end{split}
\end{equation}

Eq. \ref{eq:C_mult} allows us to re-write the inner part of the trace in Eq. \ref{eq:w_loss} as 
\begin{equation}
\label{eq:trace_term}
\begin{split}
    C_1 + C_2 - 2(C_2^{\frac{1}{2}}C_1C_2^{\frac{1}{2}})^{\frac{1}{2}} &= diag(\mathbf{\sigma}_\psi^2(\mathbf{x},\mathbf{e}_k)) + \\ diag(\mathbf{\sigma}_\psi^2(\mathbf{\hat{x}},\mathbf{e}_k)) &- 2 diag(\mathbf{\sigma}_\psi(\mathbf{x},\mathbf{e}_k)\mathbf{\sigma}_\psi(\mathbf{\hat{x}},\mathbf{e}_k))\\
    = diag(\mathbf{\sigma}_\psi^2(\mathbf{x},\mathbf{e}_k)) + \mathbf{\sigma}_\psi^2(&\mathbf{\hat{x}},\mathbf{e}_k) - 2\mathbf{\sigma}_\psi(\mathbf{x},\mathbf{e}_k)\mathbf{\sigma}_\psi(\mathbf{\hat{x}},\mathbf{e}_k))\\
    = diag((\mathbf{\sigma}_\psi(\mathbf{x},\mathbf{e}_k) &- \mathbf{\sigma}_\psi(\mathbf{\hat{x}},\mathbf{e}_k))^2)
    % , diag(\mathbf{\sigma}_\psi^2(\mathbf{x},\mathbf{e}_k))
\end{split}
\end{equation}

Substituting Eq. \ref{eq:trace_term} in Eq. \ref{eq:w_loss}, we get
\begin{equation}
\label{eq:w_loss_mod}
\begin{split}
    \mathcal{W}_2(q_{\psi}(\mathbf{z}|\mathbf{x},k), q_{\psi}(\mathbf{\hat{z}}|\mathbf{\hat{x}},k)) =& \hspace{0.2em} ||\mathbf{\mu}_\psi(\mathbf{x},\mathbf{e}_k) - \mathbf{\mu}_\psi(\mathbf{\hat{x}},\mathbf{e}_k)||_2^2\\
     + \hspace{0.2em} trace(dia&g(\mathbf{\sigma}_\psi(\mathbf{x},\mathbf{e}_k) - \mathbf{\sigma}_\psi(\mathbf{\hat{x}},\mathbf{e}_k)^2))\\
    \
    = ||\mathbf{\mu}_\psi(\mathbf{x},\mathbf{e}_k) &- \mathbf{\mu}_\psi(\mathbf{\hat{x}},\mathbf{e}_k)||_2^2 \\
    + ||\mathbf{\sigma}_\psi(\mathbf{x},\mathbf{e}_k) &- \mathbf{\sigma}_\psi(\mathbf{\hat{x}},\mathbf{e}_k)||_2^2
\end{split}
\end{equation}

\section{Qualitative Results}
\setcounter{figure}{0}
\setcounter{table}{0}
\subsection{Toy Data}
\label{ssec:app_toy}

We show the latent space learnt by our method \& GMVAE on the synthetic dataset proposed in their paper. As seen below, our clusters are tightly packed individually \& more spread overall compared to GMVAE. Good latent space separation is key for clustering as we want a representation where data is better partitioned.
\input{latex_figures/toy_data.tex}

\subsection{Generated Samples from Fashion-MNIST}
Fig. \ref{fig:gen_fashion} shows the generative ability of our method in the case of Fashion-MNIST. As it can be seen, it produces realistic images of the clusters from the dataset. Here, we show generated samples from Fashion-MNIST. Despite a little bit of overlap, each cluster almost uniquely represents a different category in the dataset, even though they are visually similar, like 'sneaker' \& 'sandal' (row 1 \& 7) or 'coat' \& 'pullover' (row 4 \& 5). This shows the discriminatory power of our learnt latent space.
\begin{figure}[h!]
    \centering
    \includegraphics[width=0.5\textwidth]{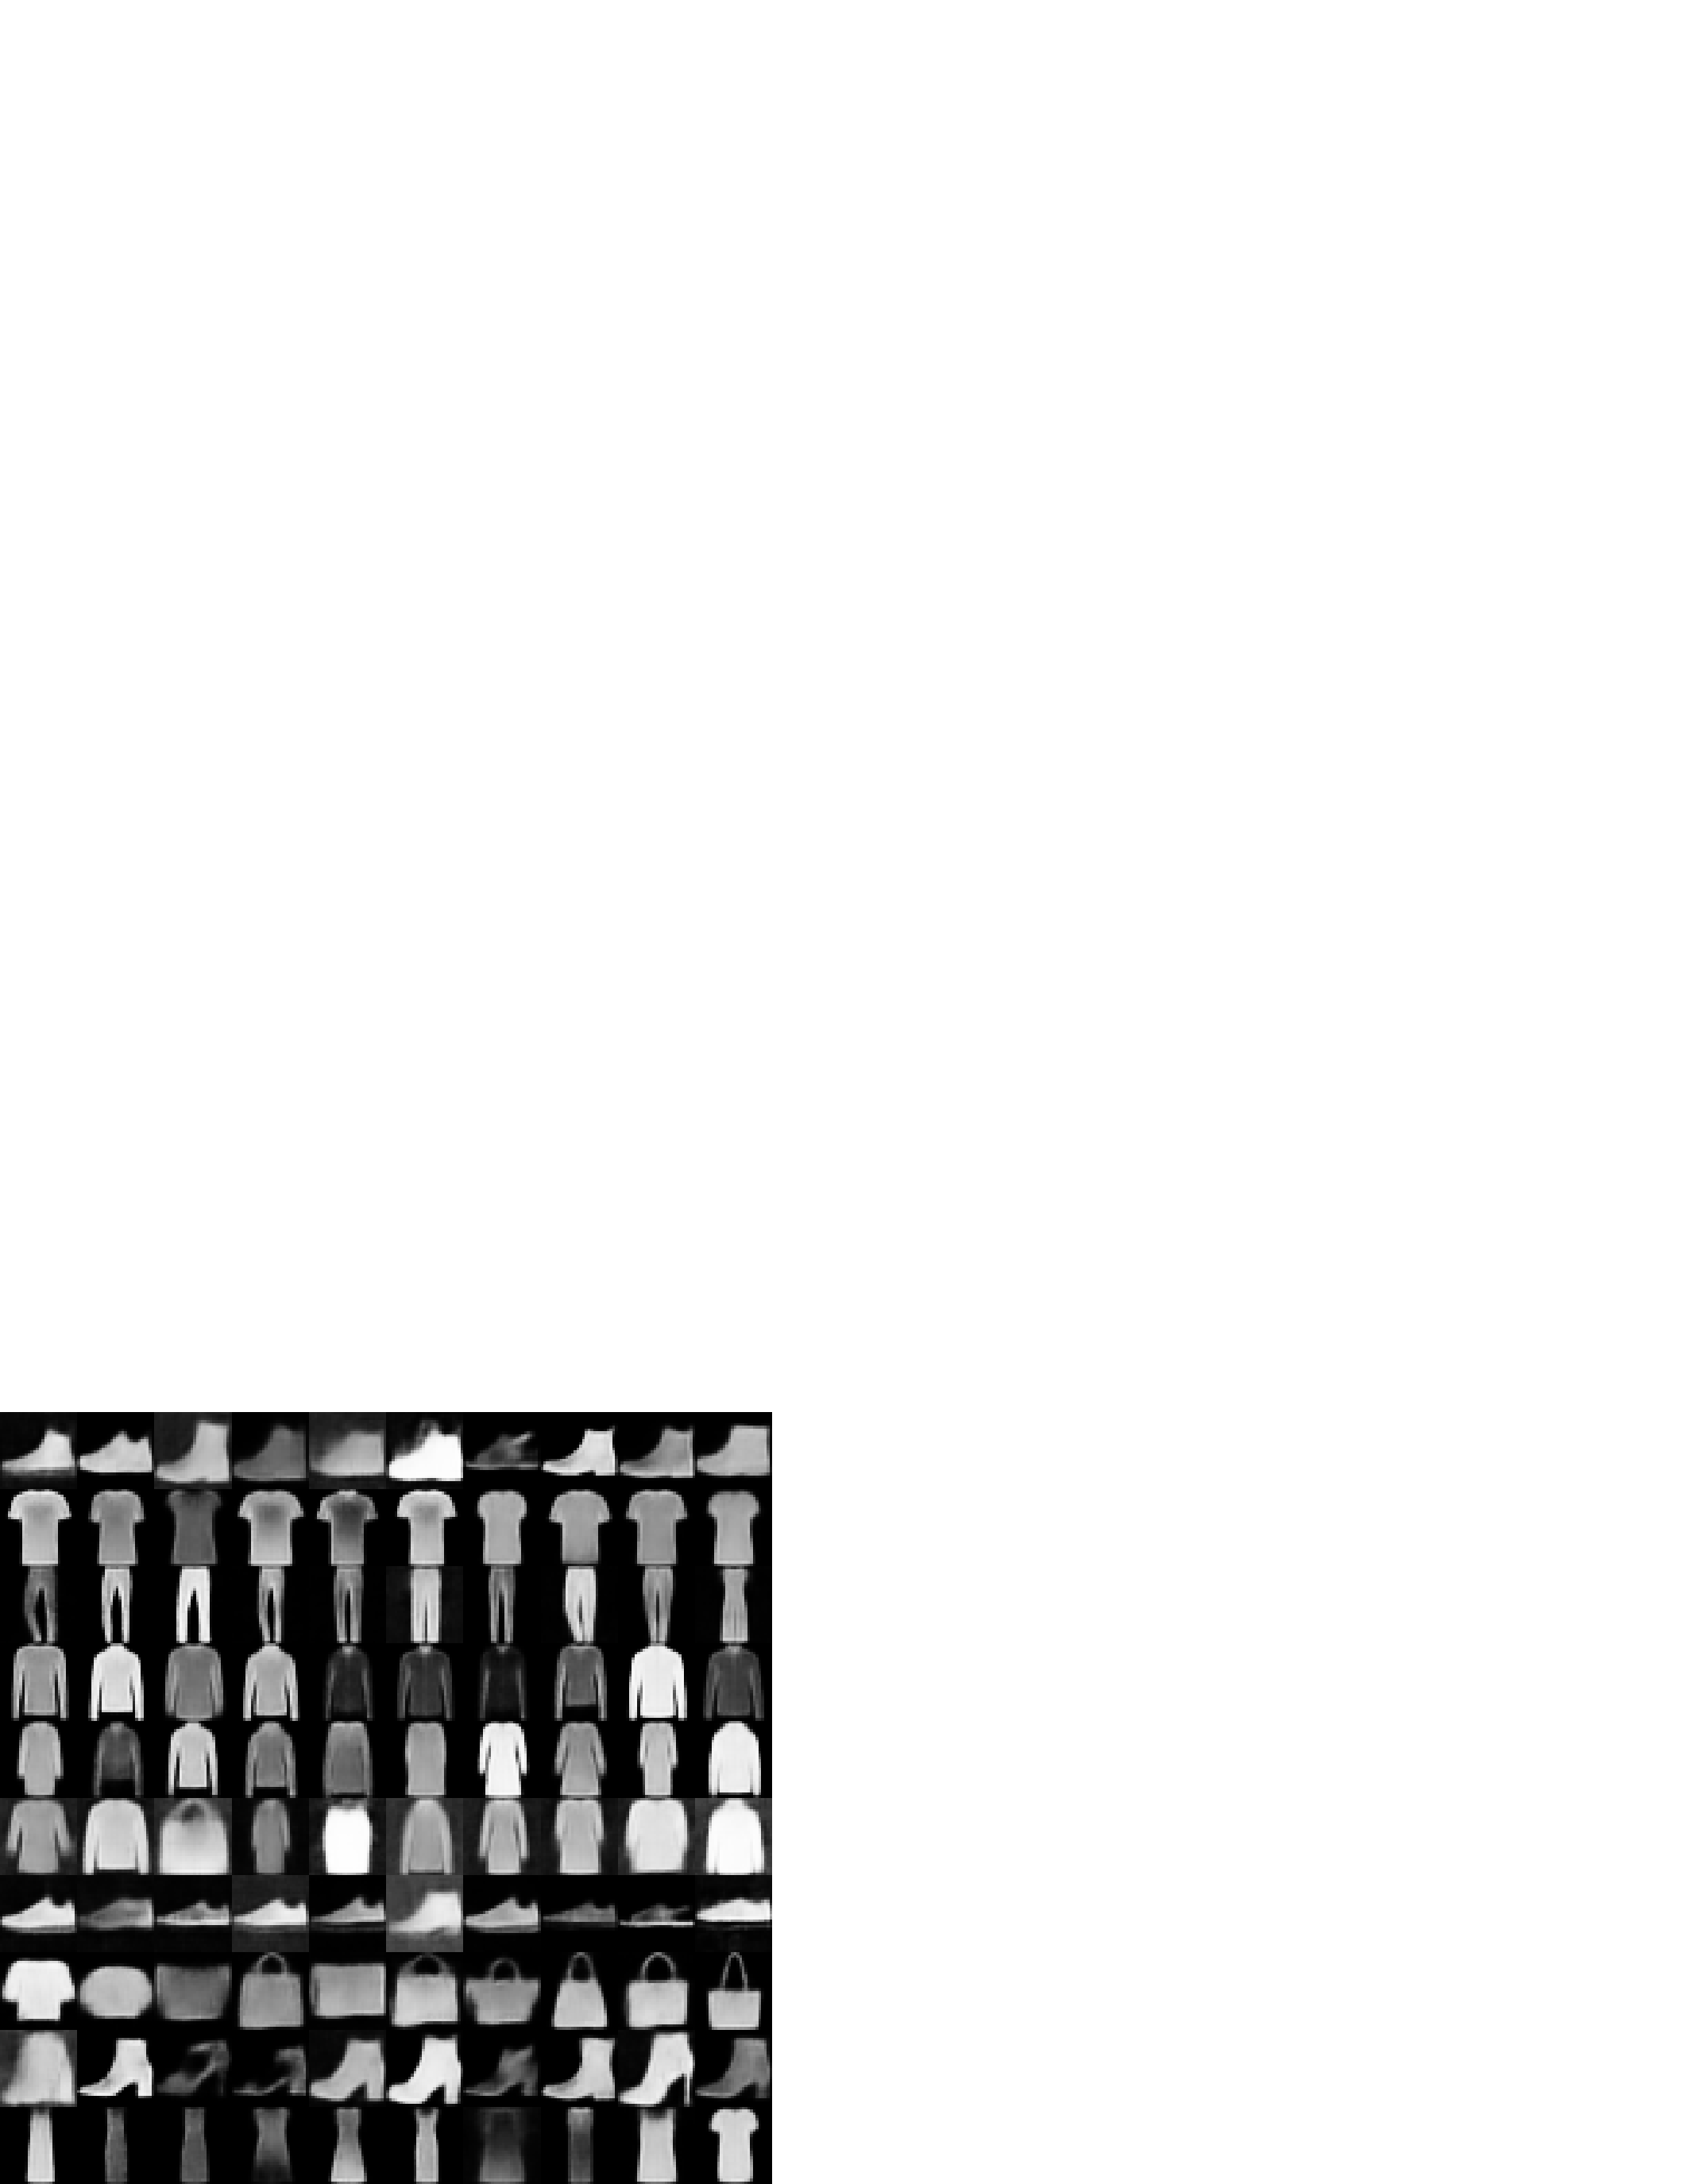}
    \caption{Images generated from each of the clusters in Fashion-MNIST. Each row represents a cluster and each column is an independent Bernoulli distribution generated by $p_\theta(\mathbf{x}|\mathbf{z})$ given a latent $\mathbf{z}$ sampled from the Gaussian Distribution $p_\beta(\mathbf{z}|k)$ corresponding to the $k^{th}$ cluster.}
    \label{fig:gen_fashion}
\end{figure}

\subsection{Best images from STL-10}
In order to see how well our method clusters high dimensional data, we take a look at the top 10 images corresponding to each cluster for STL-10. From Fig. \ref{fig:stl-best} it can be seen that our method is able to distinguish well between similar classes like 'cat' \& 'dog' (row 4 \& 6) and between 'aeroplane' \& 'bird' (row 1 \& 2) where the background is the same (sky) and the structure is similar (head, wings, tail).
\begin{figure}[h!]
    \centering
    \includegraphics[width=0.5\textwidth]{images/stl_best10.png}
    \caption{The top 10 images having highest probability for belonging to each cluster in STL-10.}
    \label{fig:stl-best}
\end{figure}

\section{Cluster visualization}
\label{sec:app_clusters}
\setcounter{figure}{0}
\setcounter{table}{0}
To see how well the clusters are separated in the latent space, we visualize the means of the posterior and the prior using t-SNE. The posterior representation of a subset of testing images can be seen in Fig. \ref{fig:tsne_post}. For the prior, we randomly generate 500 samples from each cluster, to see how well the prior has been learnt. This can be seen in Fig. \ref{fig:tsne_prior}. Evidently, we can see a clear separation between clusters from the beginning itself (11 epochs), which gets refined as the iterations go on. This not only shows the discriminatory nature of the learnt representations, but also the speed with which it becomes a characteristic of the latent space. The colour coding for the visualization is given in Fig. \ref{fig:colour_coding}.

\input{latex_figures/tsne_post.tex}
\input{latex_figures/tsne_prior.tex}

\begin{figure}[h!]
    \centering
    \includegraphics[width=0.1\textwidth]{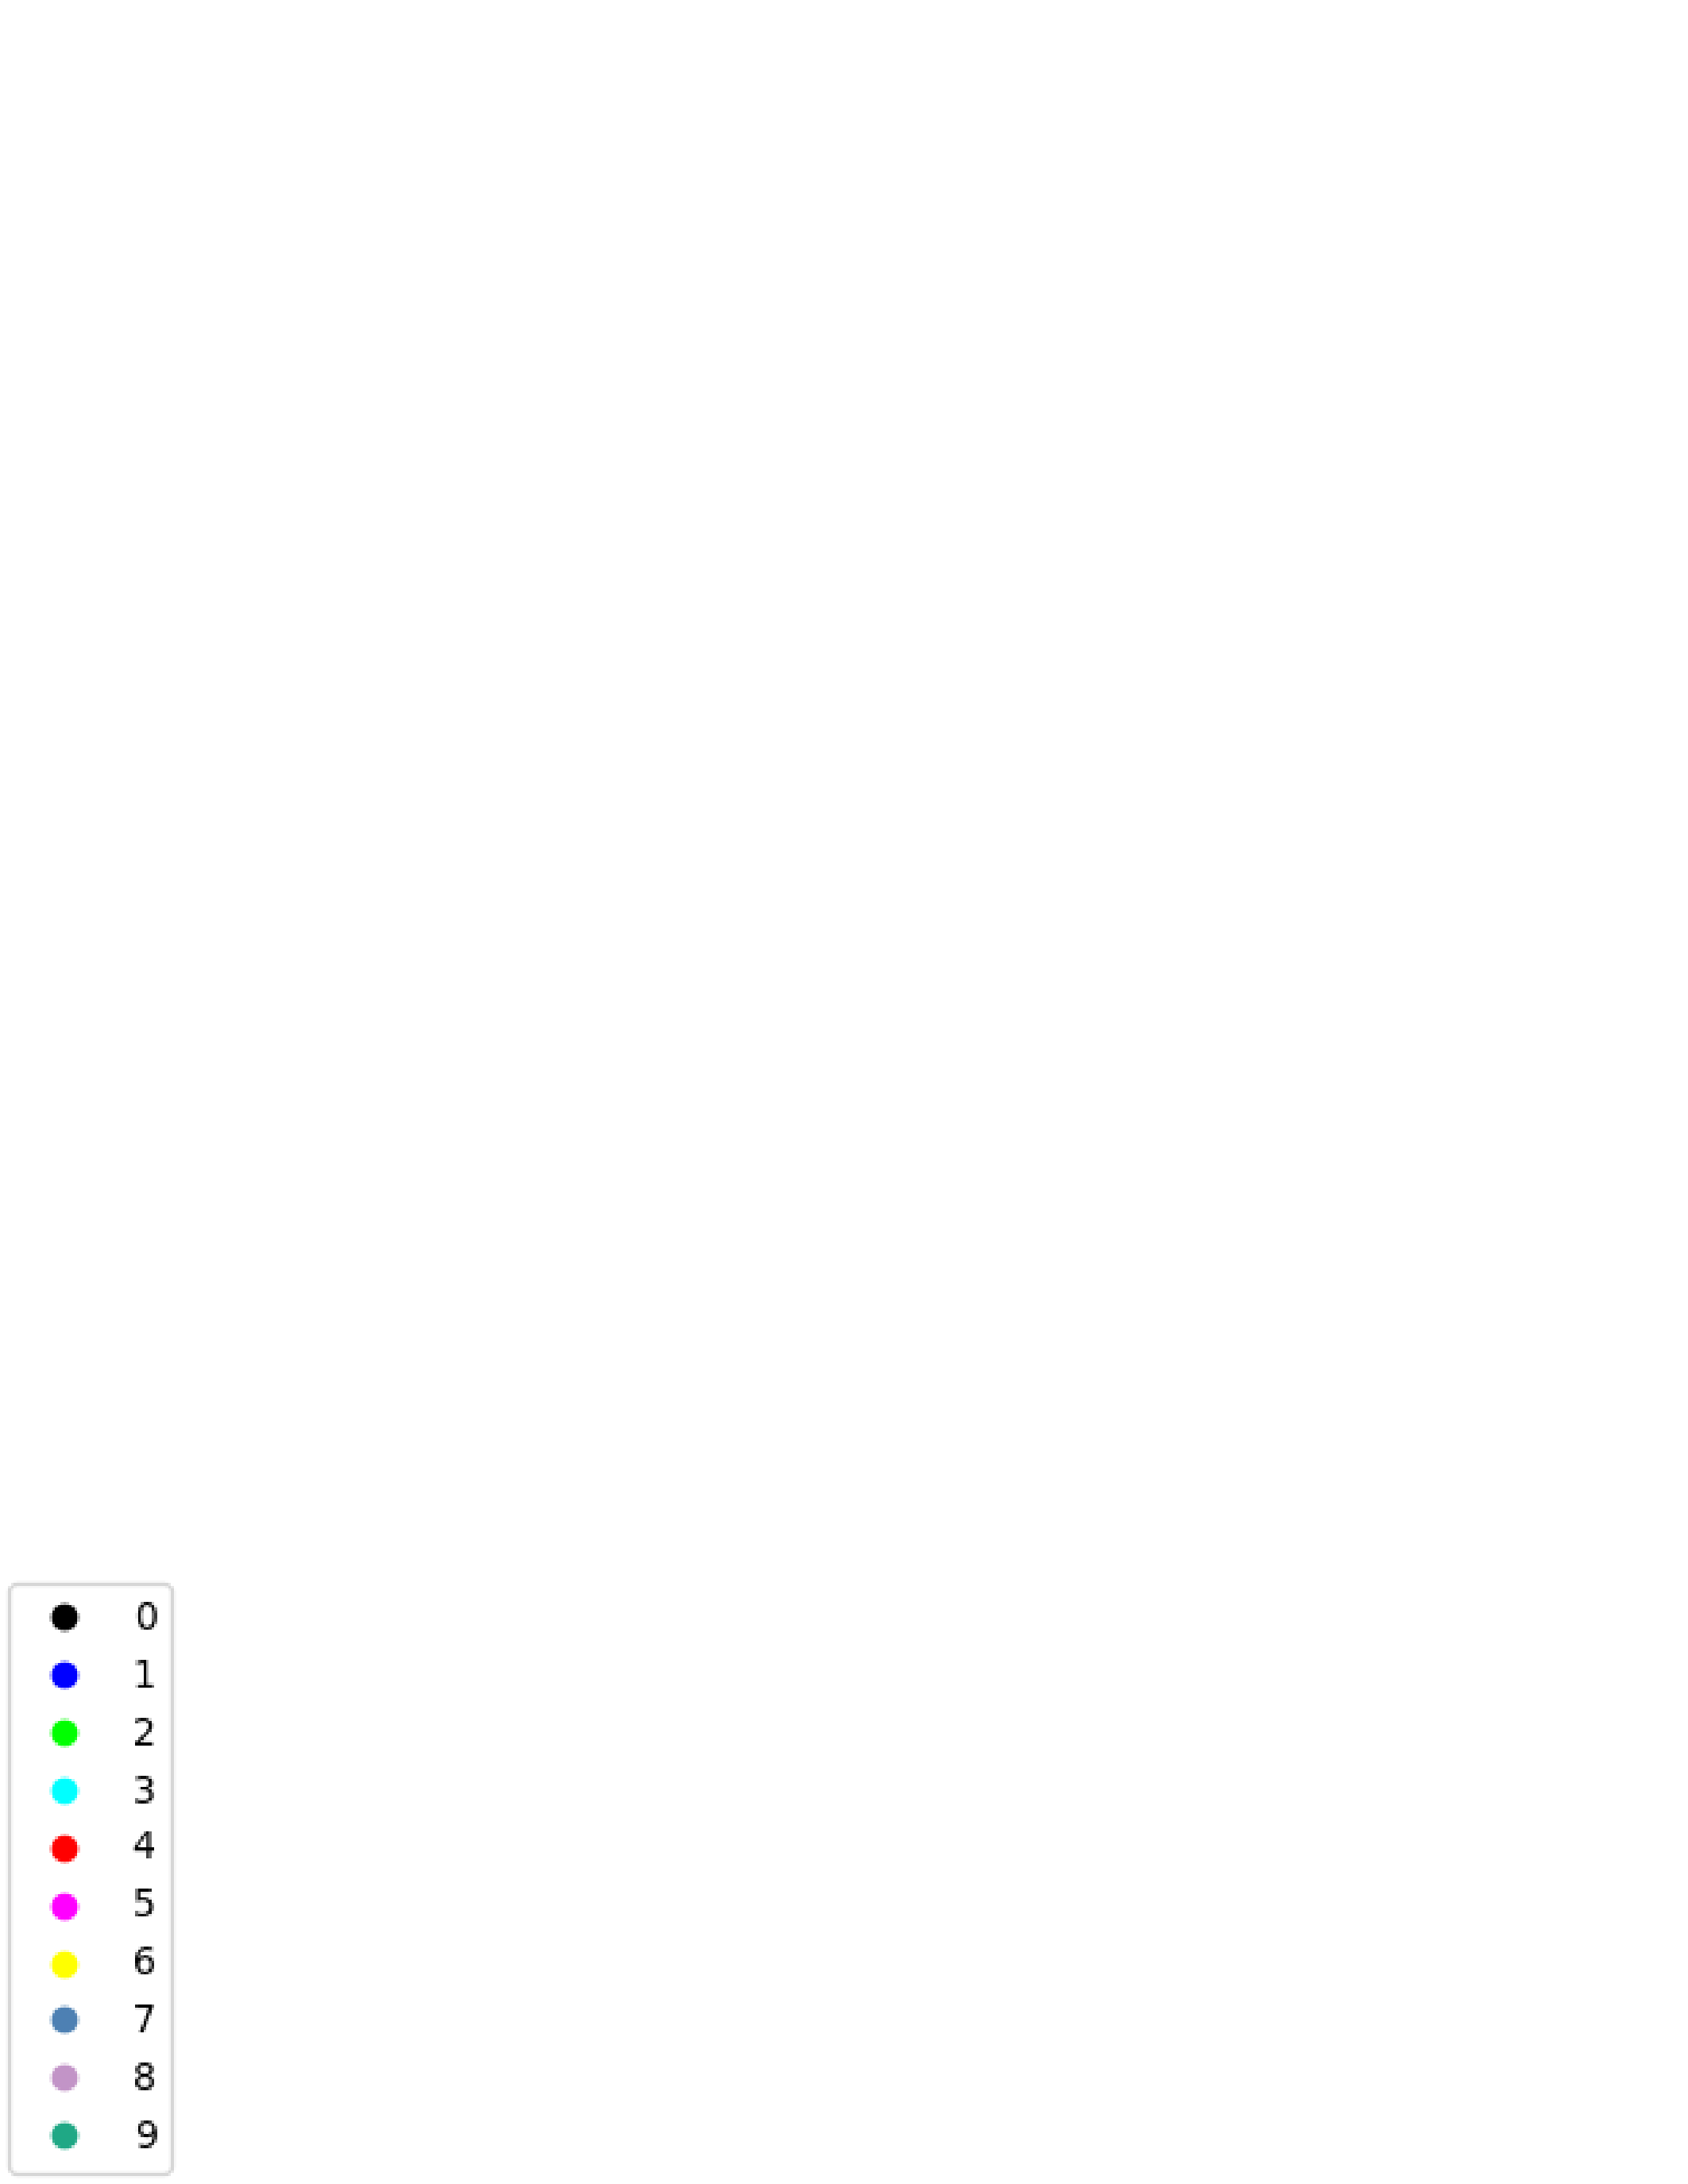}
    \caption{Colour coding used to represent digits in t-SNE visualization}
    \label{fig:colour_coding}
\end{figure}

% \section{Imbalanced clusters}
% \label{sec:app_imbalanced}
% \setcounter{figure}{0}
% \setcounter{table}{0}
% In order to study the performance of our method on imbalanced data, we follow the same imbalanced sampling mechanism as in DEC. We define a minimum retention rate $r_{min}$, which is the probability with which samples of class 0 will be retained. Samples of class 9 are retained with probability 1 and the retention rate for the other classes vary linearly from $r_{min}$ to 1. Therefore, the ratio of the size of the largest and smallest cluster would be $1/r_{min}$. The performance of our method on imbalanced sampling can be seen in Table \ref{tab:imbalanced}. 
% \input{latex_tables/imbalanced.tex}

\section{Latent Space Interpolation}
\setcounter{figure}{0}
\setcounter{table}{0}
\input{appendix/interp.tex}

\section{Ablation Study}
\label{sec:app_ablation}
\setcounter{figure}{0}
\setcounter{table}{0}
We perform an ablation study by observing the effect on each of our proposed additions individually on a vanilla implementation of the VAE with a Gaussian Mixture prior. We also see the effect of varying the reconstruction scale factor, as mentioned in the ending of Sec. {\color{red} 4.3}. The results for this study are given in Table \ref{tab:ablation}. As it can be seen, our vanilla method itself performs decently. Adding just the scale-factor for STL-10 helps improve the accuracy. Just adding the $L2$ loss increases the accuracy by a small margin, while adding the $\mathcal{W}_2$ loss increases it by a larger margin. This shows that enforcing a consistent latent space representation helps make the learning more robust. Finally, we get the best performance by combining all our additions together. 
\input{latex_tables/ablation.tex}
