# Supplementary material for: Variational Clustering: Leveraging Variational Autoencoders for Image Clustering
Source: arXiv:2005.04613 source file (2020-05-10)
Supplement: Supplementary file 3 [file augmentation.tex]

The augmentation loss can be written as:
\begin{equation}
\label{eq:aug_loss}
\begin{split}
    \mathcal{L}_{aug} = \sum_{k=1}^K||q_{\phi}(k|\mathbf{x}) - q_{\phi}(k|\mathbf{\hat{x}})||_2^2 \\
    + \mathbb{E}_{q_{\phi}(k|\mathbf{x})}[\mathcal{W}_2(q_{\psi}(\mathbf{z}|\mathbf{x},k), q_{\psi}(\mathbf{\hat{z}}|\mathbf{\hat{x}},k))]
\end{split}
\end{equation}

where $\mathcal{W}_2$ is the 2-Wasserstein distance between the predicted posteriors. The expectation in the latter is due to the fact that we do not know the ground truth cluster to reduce the distance between the prior and posterior of that cluster. Instead, taking the expectation allows us to give a higher weight to the cluster it's predicted to belong to and a lower weight for clusters that are not associated with the given image. 
The 2-Wasserstein distance between the predicted posteriors has a closed form solution\cite{dowson1982frechet} since they are Gaussian distributions, which is given by

\begin{equation}
\label{eq:w_loss}
\begin{split}
    \mathcal{W}_2(q_{\psi}(\mathbf{z}|x,k), q_{\psi}(\mathbf{\hat{z}}|\mathbf{\hat{x}},k)) = ||\mathbf{\mu}_\psi(\mathbf{x},\mathbf{e}_k) - \mathbf{\mu}_\psi(\mathbf{\hat{x}},\mathbf{e}_k)||_2^2\\
     + \hspace{0.2em} trace(C_1 + C_2 - 2(C_2^{\frac{1}{2}}C_1C_2^{\frac{1}{2}})^{\frac{1}{2}})
    % , diag(\mathbf{\sigma}_\psi^2(\mathbf{x},\mathbf{e}_k))
\end{split}
\end{equation}

with $C_1 = diag(\mathbf{\sigma}_\psi^2(\mathbf{x},\mathbf{e}_k))$ and $C_2 = diag(\mathbf{\sigma}_\psi^2(\mathbf{\hat{x}},\mathbf{e}_k))$ in our case. Given this form of $C_1$ and $C_2$, we can simplify $(C_2^{\frac{1}{2}}C_1C_2^{\frac{1}{2}})^{\frac{1}{2}}$ as 
\begin{equation}
\label{eq:C_mult}
\begin{split}
(C_2^{\frac{1}{2}}C_1C_2^{\frac{1}{2}})^{\frac{1}{2}} &= diag(\mathbf{\sigma}_\psi(\mathbf{\hat{x}},\mathbf{e}_k)\mathbf{\sigma}_\psi^2(\mathbf{x},\mathbf{e}_k)\mathbf{\sigma}_\psi(\mathbf{\hat{x}},\mathbf{e}_k))^{\frac{1}{2}}\\
&= diag(\mathbf{\sigma}_\psi(\mathbf{x},\mathbf{e}_k)\mathbf{\sigma}_\psi(\mathbf{\hat{x}},\mathbf{e}_k))
\end{split}
\end{equation}

Eq. \ref{eq:C_mult} allows us to re-write the inner part of the trace in Eq. \ref{eq:w_loss} as 
\begin{equation}
\label{eq:trace_term}
\begin{split}
    C_1 + C_2 - 2(C_2^{\frac{1}{2}}C_1C_2^{\frac{1}{2}})^{\frac{1}{2}} &= diag(\mathbf{\sigma}_\psi^2(\mathbf{x},\mathbf{e}_k)) + \\ diag(\mathbf{\sigma}_\psi^2(\mathbf{\hat{x}},\mathbf{e}_k)) &- 2 diag(\mathbf{\sigma}_\psi(\mathbf{x},\mathbf{e}_k)\mathbf{\sigma}_\psi(\mathbf{\hat{x}},\mathbf{e}_k))\\
    = diag(\mathbf{\sigma}_\psi^2(\mathbf{x},\mathbf{e}_k)) + \mathbf{\sigma}_\psi^2(&\mathbf{\hat{x}},\mathbf{e}_k) - 2\mathbf{\sigma}_\psi(\mathbf{x},\mathbf{e}_k)\mathbf{\sigma}_\psi(\mathbf{\hat{x}},\mathbf{e}_k))\\
    = diag((\mathbf{\sigma}_\psi(\mathbf{x},\mathbf{e}_k) &- \mathbf{\sigma}_\psi(\mathbf{\hat{x}},\mathbf{e}_k))^2)
    % , diag(\mathbf{\sigma}_\psi^2(\mathbf{x},\mathbf{e}_k))
\end{split}
\end{equation}

Substituting Eq. \ref{eq:trace_term} in Eq. \ref{eq:w_loss}, we get
\begin{equation}
\label{eq:w_loss_mod}
\begin{split}
    \mathcal{W}_2(q_{\psi}(\mathbf{z}|\mathbf{x},k), q_{\psi}(\mathbf{\hat{z}}|\mathbf{\hat{x}},k)) =& \hspace{0.2em} ||\mathbf{\mu}_\psi(\mathbf{x},\mathbf{e}_k) - \mathbf{\mu}_\psi(\mathbf{\hat{x}},\mathbf{e}_k)||_2^2\\
     + \hspace{0.2em} trace(dia&g(\mathbf{\sigma}_\psi(\mathbf{x},\mathbf{e}_k) - \mathbf{\sigma}_\psi(\mathbf{\hat{x}},\mathbf{e}_k)^2))\\
    \
    = ||\mathbf{\mu}_\psi(\mathbf{x},\mathbf{e}_k) &- \mathbf{\mu}_\psi(\mathbf{\hat{x}},\mathbf{e}_k)||_2^2 \\
    + ||\mathbf{\sigma}_\psi(\mathbf{x},\mathbf{e}_k) &- \mathbf{\sigma}_\psi(\mathbf{\hat{x}},\mathbf{e}_k)||_2^2
\end{split}
\end{equation}
